# Supplementary material for: Room-temperature quantum emission from interface excitons in mixed-dimensional heterostructures
Source: arXiv:2307.15399 ancillary file (2023-07-28)
Supplement: Supplementary file 1 [file SI.pdf]

**Supplementary Information**

# Room-temperature quantum emission from interface excitons in mixed-dimensional heterostructures

Nan Fang[1,*], Yih-Ren Chang[1], Shun Fujii[2,3], Daiki Yamashita[2,4], Mina Maruyama[5], Yanlin Gao[5], Chee Fai Fong[1], Daichi Kozawa[1,2,6], Keigo Otsuka[1,7], Kosuke Nagashio[8], Susumu Okada[5], Yuichiro K. Kato[1,2,*]

[1]Nanoscale Quantum Photonics Laboratory, RIKEN Cluster for Pioneering Research, Saitama 351-0198, Japan

[2]Quantum Optoelectronics Research Team, RIKEN Center for Advanced Photonics, Saitama 351-0198, Japan

[3]Department of Physics, Keio University, Yokohama 223-8522, Japan

[4]Platform Photonics Research Center, National Institute of Advanced Industrial Science and Technology (AIST), Ibaraki 305-8568, Japan

[5]Department of Physics, University of Tsukuba, Ibaraki 305-8571, Japan

[6]Research Center for Materials, National Institute for Materials Science, Ibaraki 305-0044, Japan

[7]Department of Mechanical Engineering, The University of Tokyo, Tokyo 113-8656, Japan

[8]Department of Materials Engineering, The University of Tokyo, Tokyo 113-8656, Japan

* email: nan.fang@riken.jp, yuichiro.kato@riken.jp

## Supplementary Note 1:
## Layer number dependence of PL from suspended $WSe_2$ flakes

The PL from the suspended $WSe_2$ flakes displays two primary peaks that vary with the layer number, which are assigned to A exciton and indirect exciton (IDX). As illustrated in Supplementary Fig. 1, the peak energy of IDX is more sensitive to the layer number than that of the A exciton, which is consistent with previous studies [1]. It is worth noting that the PL emission from the $WSe_2$ flakes is at a significantly higher energy than the newly observed IX peaks.

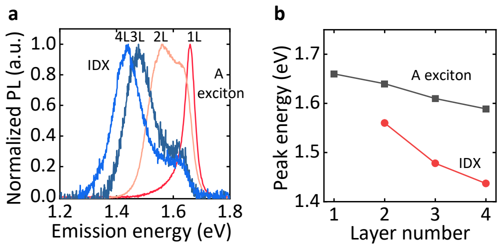


**Supplementary Fig. 1 | Layer-number dependent PL spectra from the suspended $WSe_2$ flakes. a**, PL spectra from the suspended $WSe_2$ flakes with different layer numbers. The excitation power is 10 $\mu$W. **b**, The extracted A exciton and IDX peak energies as a function of the $WSe_2$ layer number.

## Supplementary Note 2:
## Temporal evolution of PL in a CNT/$WSe_2$ heterostructure

The PL emission showcases a significant temporal evolution before the stable interface excitons form. Supplementary Fig. 2a illustrates a time trace of PL from a freshly prepared (9,4) CNT/2L $WSe_2$ sample. Two peaks, $E_{11}$ (1.112 eV) and $E_K$ (0.975 eV) are clearly observed, where $E_K$ corresponds to the K-momentum exciton. In addition, new peaks sporadically appear at various energies, which are attributed to interface excitons. The representative PL spectra are shown in Supplementary Fig. 2b. The eight IXs, located at energies of 0.825, 1.069, 0.881, 1.006, 0.964, 0.920, 0.804, and 0.859 eV, are labeled as $IX_{1-1}$ to $IX_{1-8}$, respectively. Among them, only $IX_{1-1}$ stabilizes after this extended time trace measurement of PL, while others disappear. The $IX_{1-1}$ peak exhibits remarkable air stability over a period of 121 days (Supplementary Fig. 2c), likely due to the chemical inertness of both CNTs and $WSe_2$.

To gain more insight, we plot the time-trace of PL intensity for each IX (Supplementary Fig. 2d). First, PL from most IXs show abrupt blinking over time, with $IX_{1-1}$ and $IX_{1-7}$ displaying a near "on" and "off" blinking noise. Such pure two-level blinking behavior has been primarily reported in highly confined 0D systems like quantum dots [2] and single molecules [3], suggesting that the interface states here tend to be single emitters. Second, $IX_{1-2}$ and $IX_{1-4}$ correlate with $E_{11}$ when blinking, while other IXs exhibit no clear correlations, implying different origins among the diverse IXs. Third, the blinking of IXs occurs on a scale of tens of seconds, indicative of a slow process. This temporal evolution of PL differs from photobleaching in single molecules originating from chemical reaction [4]. We suspect the observed PL evolution could be related to charge and/or atomic registry. If so, $IX_{1-1}$ could originate from a stable state with a specific configuration, while others represent metastable states that dissipate over time. The atomic reconstruction has been widely observed in 2D-2D heterostructures [5]. In our CNT/$WSe_2$ samples, the atomic reconstruction is expected to be strong due to the absence of a substrate.

# Supplementary information

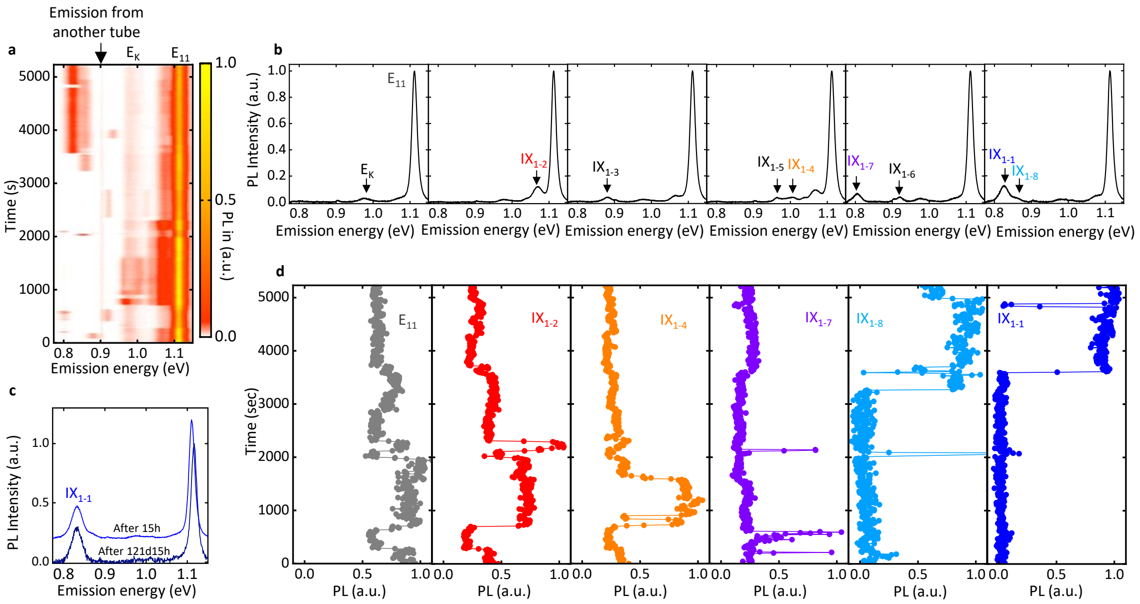

**Supplementary Fig. 2 | PL evolution of interface excitons. a**, Time-trace PL of the (9,4) CNT/2L $WSe_2$ sample shown in Fig. 4. A weak emission peak at 0.903 eV comes from the $E_{11}$ emission of an adjacent CNT. The excitation energy is adjusted to $E_{22}$ of 1.70 eV and the power is 5 $\mu$W. **b**, PL spectra at different times showing various IXs. **c**, PL spectra after 15 hours (blue) and after 121 days (black) from the formation of the heterostructure in order to demonstrate a long-scale stability of $IX_{1\text{-}1}$. **d**, Time-trace of the integrated PL intensity for different IX peaks, extracted from **a**. The excitation energy is adjusted to $E_{22}$ of 1.70 eV and the power is 10 $\mu$W for (**a**,**b**,**c**) and 5 $\mu$W for (**c**).

## Supplementary Note 3:
## A broad PL map of a low-energy interface exciton

Supplementary Fig. 3 shows an integrated PL image from the $IX_2$ peak. The image center is precisely at the position of $E_{11}$ and $IX_1$ peaks as shown in Fig.1 g,h. We note that the image is enlarged because of a strong power saturation behavior of $IX_2$ peak (Fig. 3c,d) and a fringe pattern from the optical system.

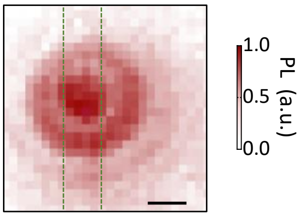


**Supplementary Fig. 3 | An enlarged PL map of an interface exciton. a**, A PL intensity map of $IX_2$ for the (9,4) CNT/1L $WSe_2$ sample shown in Fig.1. The excitation energy is 1.653 eV and excitation power is 10 $\mu$W. The edge of the trench is indicated by the green broken line. The scale bar represents 1 $\mu$m.

## Supplementary Note 4:
## Emission polarization angle in other samples

The emission polarization from the (9,4) CNT/1L $WSe_2$ sample (Fig. 3a) reveals an angle difference between the $E_{11}$ exciton and the interface excitons. Here we focus on (9,4) CNT/2L $WSe_2$ heterostructures to further investigate such deviation. Supplementary Fig. 4a is taken from the sample shown in Supplementary Fig. 2, and the polarization angle of $IX_{1\text{-}1}$ has a slight deviation from that of $E_{11}$ by 7.1°. Another prepared (9,4) CNT/2L $WSe_2$ sample exhibits three interface excitons at energies of 1.056, 0.823, and 0.801 eV (Supplementary Fig. 5a,b), and are labeled as $IX_{2\text{-}1}$, $IX_{2\text{-}2}$, and $IX_{2\text{-}3}$, respectively. The polarization angle of $IX_{2\text{-}1}$, $IX_{2\text{-}2}$, and $IX_{2\text{-}3}$ clearly deviates from that of $E_{11}$, with values of 21.0°, 17.8°, and 20.4°, respectively. Such variations in the polarization angle cannot be solely explained by artifacts of the optical system, but suggesting the distinct distortions of interfacial dipoles in different samples.

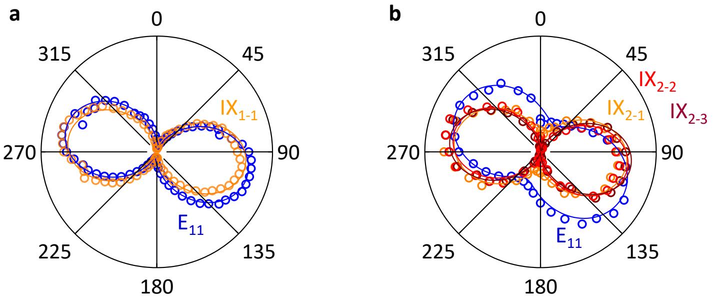


**Supplementary Fig. 4 | Emission polarization measurements in (9,4) CNT/2L $WSe_2$ samples. a**, Emission polarization dependence of PL emission from $E_{11}$ (blue circles) and $IX_{1\text{-}1}$ (orange circles). The lines are fits to a cosine squared function. The excitation energy is 1.699 eV and excitation power is 4 $\mu$W. **b**, Emission polarization dependence of PL emission from $E_{11}$ (blue circles), $IX_{2\text{-}1}$ (orange circles), $IX_{2\text{-}2}$ (red circles), and $IX_{2\text{-}3}$ (wine circles). The lines are fits to a cosine squared function. The excitation energy is 1.669 eV and excitation power is 1 $\mu$W.

## Supplementary Note 5:
## Laser power saturation behaviors in IXs

The IXs shown in Fig. 3 are strongly confined, as characterized by the power dependence of the PL spectra. In other samples where interface excitons are also observed, we note that the saturation behavior depends on the energy difference between $E_{11}$ and interface excitons.

PL spectra taken from the (9,4)/2L $WSe_2$ sample at powers of 0.2 $\mu$W and 2 $\mu$W are shown in Supplementary Fig. 5a,b. Power dependence of the integrated PL for each peak is plotted in Supplementary Fig. 5c. The $E_{11}$ peak located at 1.099 eV exhibits quasi-linear power dependence. The $IX_{2-1}$ peak, with energy close to $E_{11}$, shows similar power dependence. In contrast, a clear saturation behavior is observed for the low-energy $IX_{2-2}$ and $IX_{2-3}$ peaks. Such a peak-energy dependent saturation behavior can be caused by the different trap potentials in IXs, and in which case $IX_{2-2}$ and $IX_{2-3}$ would have large potentials that result in strong confinement. In comparison, $IX_{2-1}$ could be weakly confined due to a shallow potential.

Similar energy-dependent power saturation is also confirmed in other samples, as shown in Supplementary Fig. 5d-r. Low-energy $IX_{1-1}$, $IX_{3-2}$, and $IX_{3-3}$ peaks show substantial saturation behavior. In contrast, high-energy peaks near $E_{11}$ such as $IX_{4-1}$, $IX_{5-1}$, $IX_{6-1}$, and $IX_{6-2}$ exhibit similar power dependence with $E_{11}$ and $E_K$. These IXs could be highly delocalized, and we do not expect single-photon emission from these states (see Supplementary Fig. 8).

# Supplementary information

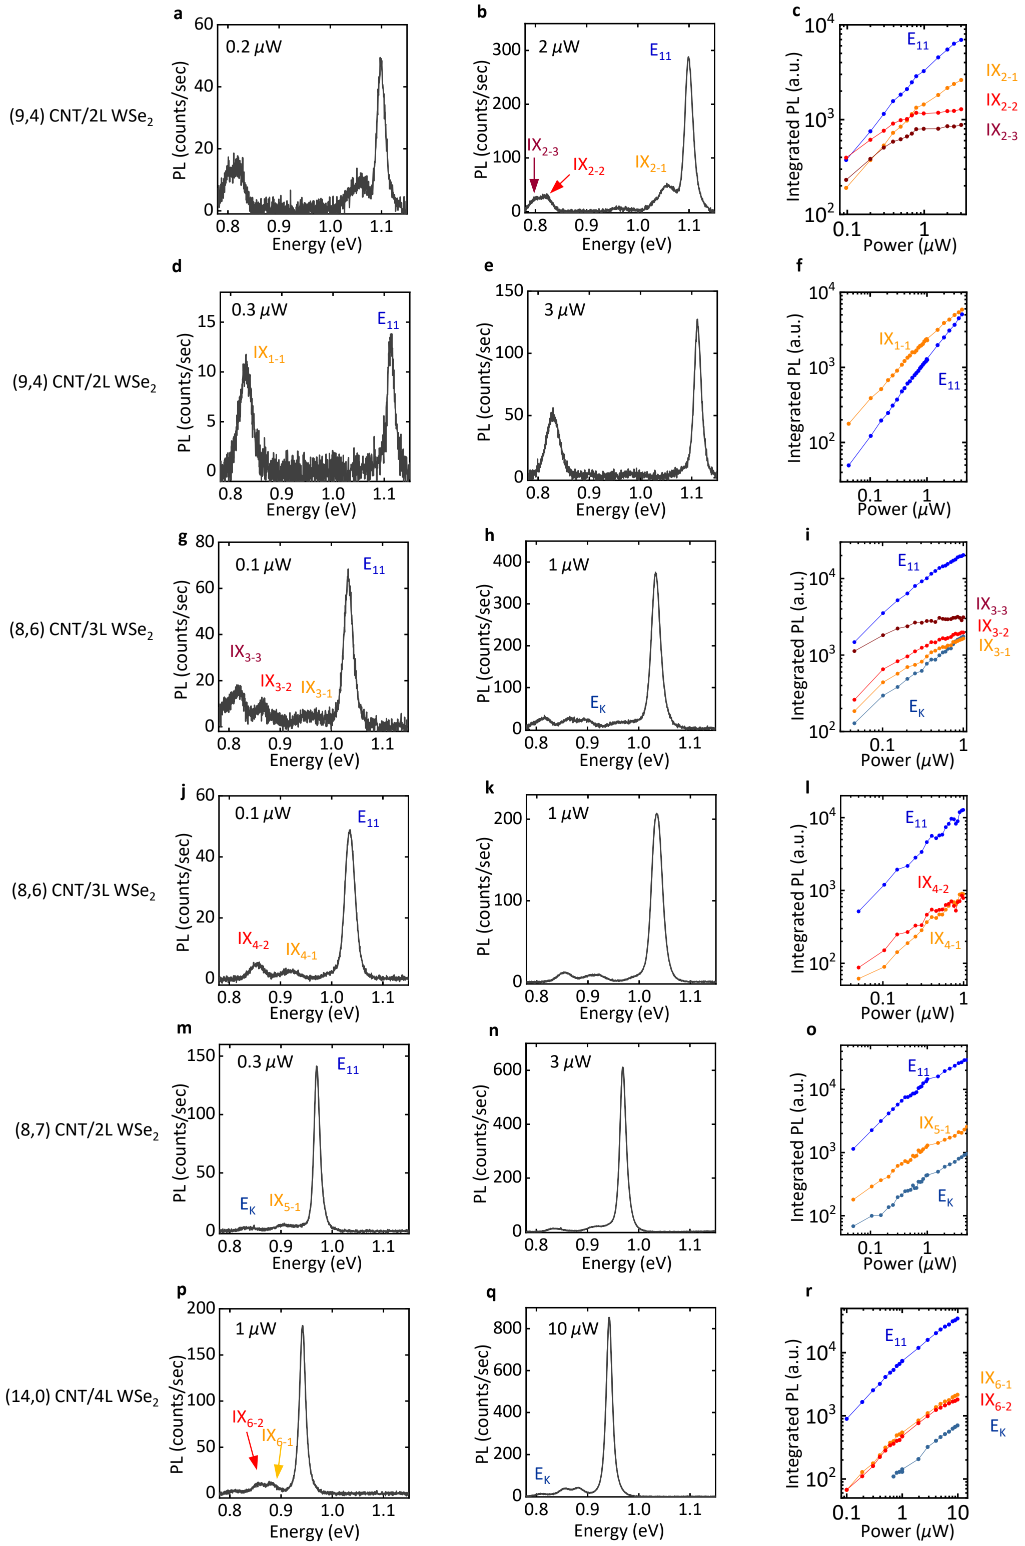

**Supplementary Fig. 5 | Laser power dependence of IXs in different samples. a-c,** PL spectra for the (9,4) CNT/2L $WSe_2$ sample shown in Supplementary Fig. 4b at powers of 0.2 $\mu$W (**a**) and 2 $\mu$W (**b**). (**c**) The laser power dependence of the integrated intensity for the different PL peaks in (**a**,**b**). **d-f,** PL spectra for the (9,4) CNT/2L $WSe_2$ sample shown in Supplementary Fig. 2 at powers of 0.3 $\mu$W (**d**) and 3 $\mu$W (**e**). (**f**) The laser power dependence of the integrated intensity for the different PL peaks in (**d**,**e**). **g-i,** PL spectra for the (8,6) CNT/3L $WSe_2$ sample shown in Fig. 2a at powers of 0.1 $\mu$W (**g**) and 1 $\mu$W (**h**). (**i**) The laser power dependence of the integrated intensity for the different PL peaks in (**g**,**h**). **j-l,** PL spectra for another (8,6) CNT/3L $WSe_2$ sample at powers of 0.1 $\mu$W (**j**) and 1 $\mu$W (**k**). (**l**) The laser power dependence of the integrated intensity for the different PL peaks in (**j**,**k**). **m-o,** PL spectra for the (8,7) CNT/2L $WSe_2$ sample shown in Fig. 2a at powers of 0.3 $\mu$W (**m**) and 3 $\mu$W (**n**). (**o**) The laser power dependence of the integrated intensity for the different PL peaks in (**m**,**n**). **p-r,** PL spectra for the (14,0) CNT/4L $WSe_2$ sample shown in Fig. 2a at powers of 1 $\mu$W (**p**) and 10 $\mu$W (**q**). (**r**) The laser power dependence of the integrated intensity for the different PL peaks in (**p**,**q**). Excitation energy is adjusted to $E_{22}$ for each heterostructure.

## Supplementary Note 6:
## Abrupt blinking noise from IXs

Most low-energy peaks show near "on" and "off" two-state blinking noise. Here we demonstrate the long time scale PL trace of an IX peak from another prepared (9,4) CNT/2L $WSe_2$ sample, which exhibits several transitions. The unstable IX peak is indicated in Supplementary Fig. 6a. The PL trace from this peak is shown in Supplementary Fig. 6b. The PL intensity shows clear two levels and blinking over a long time scale of 20,000 s.

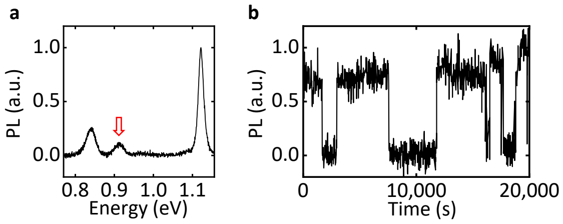


**Supplementary Fig. 6 | Long time scale PL trace of an IX peak. a,** A PL spectrum for another (9,4) CNT/2L $WSe_2$ sample. **b**, Time-trace of the IX peak as indicated by a red arrow in (**a**). The excitation energy is adjusted to 1.703 eV of $E_{22}$ and the excitation power is 5 $\mu$W.

## Supplementary Note 7:
## Background correction for second-order photon correlation results

In order to determine the intrinsic $g^{(2)}(0)$ value for interface excitons, we need to consider the effects from the uncorrelated background PL. Supplementary Fig. 7a displays the PL spectrum from the (9,4) CNT/2L $WSe_2$ heterostructure, on which photon correlation measurements in Fig.4 are conducted. In the photon correlation analysis, we subtract the background signal as indicated in the PL spectrum. Supplementary Fig. 7b presents the raw number of coincidences. The $g^{(2)}(\tau)$ shown in Fig. 4 is calculated by $g^{(2)}(\tau) = (g^{(2)}_{raw} - 1)/\rho^2 + 1$ where $g^{(2)}_{raw}$ is the normalized uncorrected correlation function [6]. Here, $\rho$ = 0.89 represents the ratio between the $IX_{1\text{-}1}$ PL intensity and the total integrated PL intensity including the background signal.

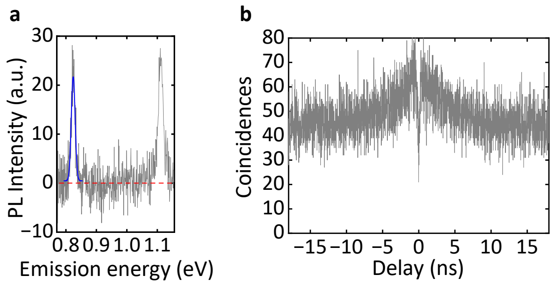


**Supplementary Fig. 7 | Raw second-order correlation results. a**, A PL spectrum from the (9,4) CNT/2L $WSe_2$ heterostructure (Supplementary Fig. 2). Peaks at 0.825 and 1.112 eV correspond to $IX_{1\text{-}1}$ and $E_{11}$, respectively. The grey line represents experimental results, while the blue line is a Gaussian fit for the $IX_{1\text{-}1}$ peak. The red dashed line indicates the 0 count level, illustrating the presence of an uncorrelated background. **b**, The raw number of coincidences in a second-order correlation measurement for the $IX_{1\text{-}1}$ PL. A longpass filter (0.886 eV) is employed to exclude PL signals from $E_{11}$.

## Supplementary Note 8:
## Second-order correlation statistics of other IX peaks

We also carry out second-order photon correlation measurements for other heterostructures. Supplementary Fig. 8a shows a PL spectrum from an (12,0) CNT/2L $WSe_2$ heterostructure, where a stable low-energy interface exciton peak $IX_{7-1}$ is observed at 0.811 eV. The second-order photon correlation measurement for this peak displays a clear antibunching dip along with a bunching peak. Moreover, the value of $g^{(2)}(0) = 0.33$ confirms the single-photon emission from this interface exciton. In the case of the (9,4) CNT/2L $WSe_2$ sample used in Supplementary Fig. 5a,b, $IX_{2-2}$ and $IX_{2-3}$ are energetically so close to each other that they cannot be separately filtered. We thus measure the correlation of the PL emission from both peaks. The statistics are shown in Supplementary Fig. 8c, and also shows an antibunching dip and a bunching peak. Compared with Fig. 4a and Supplementary Fig. 8b, the antibunching behavior here is less pronounced with $g^{(2)}(0) = 0.61$, which could be explained by the coexistence of two single-photon sources. Additionally, we conduct correlation measurements of PL emission from $IX_{6-1}$ and $IX_{6-2}$ in the (14,0) CNT/4L $WSe_2$ sample shown in Supplementary Fig. 5p,q, and neither antibunching nor bunching behavior is observed (Supplementary Fig. 8d). It is consistent with the quasi-linear power dependence of these high-energy peaks, suggesting that they are free excitons rather than trapped ones.

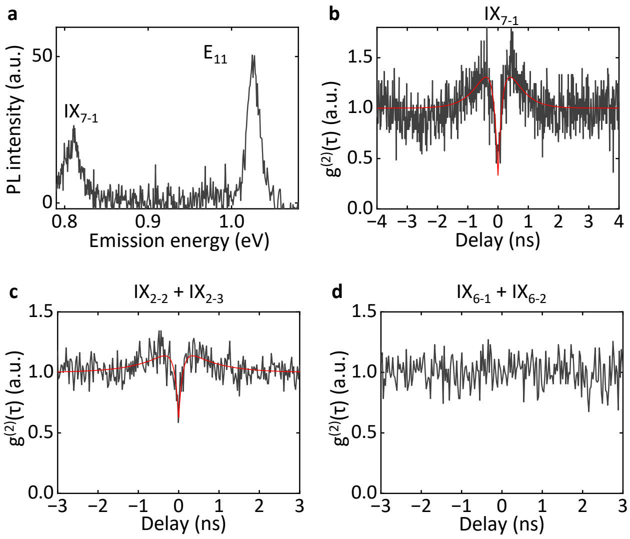


**Supplementary Fig. 8 | Second-order correlation statistics of confined and free interface excitons.** **a**, A PL spectrum from the (12,0) CNT/2L $WSe_2$ heterostructure. Peaks at 0.811 and 1.026 eV correspond to $IX_{7-1}$ and $E_{11}$, respectively. **b**, Second-order correlation statistics of $IX_{7-1}$. The excitation energy is adjusted to 1.531 eV of $E_{22}$ with a continuous-wave laser power of 0.5 $\mu$W. A longpass filter (0.826 eV) is used to collect PL emission from $IX_{7-1}$. From the fitting, we extract $\tau_A$ and $\tau_B$ as 0.295 and 0.406 ns, and

$\alpha$ and $\beta$ as 0.89 and 0.30, respectively. **c**, Second-order correlation statistics of $IX_{2\text{-}2}$ and $IX_{2\text{-}3}$ from the (9,4) CNT/2L $WSe_2$ sample. The excitation energy is adjusted to 1.664 eV of $E_{22}$ with a continuous-wave laser power of 0.4 $\mu$W. A longpass filter (0.855 eV) is used to collect PL emission from $IX_{2\text{-}2}$ and $IX_{2\text{-}3}$. From the fitting, we extract $\tau_A$ and $\tau_B$ as 0.104 and 0.757 ns, and $\alpha$ and $\beta$ as 0.51 and 0.25, respectively. **d**, Second-order correlation statistics of $IX_{6\text{-}1}$ and $IX_{6\text{-}2}$ from the (14,0) CNT/4L $WSe_2$ sample. The excitation energy is adjusted to 1.435 eV of $E_{22}$ with a continuous-wave laser power of 5 $\mu$W. A longpass filter (0.886 eV) is used to collect PL emission from $IX_{6\text{-}1}$ and $IX_{6\text{-}2}$. The grey lines are experimental results, and the red line is the fitting. The second-correlation statistics data are binned to reduce the noise. Since the background PL is small for these three samples, we do not perform background correction for the second-order correlation data.

## Supplementary References

1. Zhao, W., Ghorannevis, Z., Chu, L., Toh, M., Kloc, C., Tan, P.H. & Eda, G. Evolution of electronic structure in atomically thin sheets of $WS_2$ and $WSe_2$. *ACS Nano* **7**, 791 (2013).

2. Frantsuzov, P., Kuno, M., Janko, B. & Marcus, R. A. Universal emission intermittency in quantum dots, nanorods and nanowires. *Nat. Phys.* **4**, 519 (2008).

3. Moerner, W. E. & Orrit, M. Illuminating single molecules in condensed matter. *Science* **283**, 1670 (1999).

4. Gordon, M. P., Ha, T. & Selvin, P. R. Single-molecule high-resolution imaging with photobleaching. *Proc. Natl. Acad. Sci.* **101**, 6462 (2004).

5. Weston, A., Zou, Y., Enaldiev, V., Summerfield, A., Clark, N., Zólyomi, V., Graham, A., Yelgel, C., Magorrian, S., Zhou, M., Zultak, J., Hopkinson, D., Barinov, A., Bointon, T. H., Kretinin, A., Wilson, N. R., Beton, P. H., Fal'ko, V. I., Haigh, S. J. & Gorbachev, R. Atomic reconstruction in twisted bilayers of transition metal dichalcogenides. *Nat. Nanotechnol.* **15**, 592-597 (2020).

6. Brouri, R., Beveratos, A., Poizat, J. P. & Grangier, P. Photon antibunching in the fluorescence of individual color centers in diamond. *Opt. Lett.* **25**, 1294 (2000).
